# Supplementary material for: Variance estimation for Sequential Monte Carlo Algorithms: a backward sampling approach
Source: arXiv:2204.01401 source file (2023-01-02)
Supplement: Supplementary file 1 [file supplementary.tex]

\documentclass[bj, authoryear]{imsart}

%% Packages
\RequirePackage{amsthm,amsmath,amsfonts,amssymb}
\RequirePackage[colorlinks,citecolor=blue,urlcolor=blue]{hyperref}
\RequirePackage{graphicx}

\startlocaldefs

\usepackage{algorithm}
\usepackage{algpseudocode}
\usepackage{enumitem}
\usepackage{bm}
\usepackage{bbm}
\input{def.tex}
\usepackage{xr}
\externaldocument{mainpaper1}
% put your definitions there:
% \startlocaldefs
% \def\journal@id{~}
% \def\journal@name{~}
% \def\journal@url{~}

\newcounter{hypA}

\endlocaldefs

%%%%%%%%%%%%%%%%%%%%%%%%%%%%%%%%%%%%%%%%%%%%%%
%%                                          %%
%% Uncomment next line to change            %%
%% the type of equation numbering           %%
%%                                          %%
%%%%%%%%%%%%%%%%%%%%%%%%%%%%%%%%%%%%%%%%%%%%%%
%\numberwithin{equation}{section}
%%%%%%%%%%%%%%%%%%%%%%%%%%%%%%%%%%%%%%%%%%%%%%
%%                                          %%
%% For Axiom, Claim, Corollary, Hypothesis, %%
%% Lemma, Theorem, Proposition              %%
%% use \theoremstyle{plain}                 %%
%%                                          %%
%%%%%%%%%%%%%%%%%%%%%%%%%%%%%%%%%%%%%%%%%%%%%%
\theoremstyle{plain}

%%%%%%%%%%%%%%%%%%%%%%%%%%%%%%%%%%%%%%%%%%%%%%
%%                                          %%
%% For Assumption, Definition, Example,     %%
%% Notation, Property, Remark, Fact         %%
%% use \theoremstyle{remark}                %%
%%                                          %%
%%%%%%%%%%%%%%%%%%%%%%%%%%%%%%%%%%%%%%%%%%%%%%
\theoremstyle{remark}

\begin{document}

\title{Supplementary material for ``Variance Estimation for Sequential Monte Carlo Algorithms: a backward sampling approach''}

\begin{aug}
  \author[A]{\inits{YJ}\fnms{Yazid} \snm{Janati El Idrissi}\ead[label=e1]{yazid.janati\_elidrissi@telecom-sudparis.eu}}
  \author[B]{\inits{SL}\fnms{Sylvain} \snm{Le Corff}\ead[label=e2,mark]{\\sylvain.le\_corff@sorbonne-universite.fr}}
  \author[A]{\inits{YP}\fnms{Yohan} \snm{Petetin}\ead[label=e3,mark]{yohan.petetin@telecom-sudparis.eu}}
  %%%%%%%%%%%%%%%%%%%%%%%%%%%%%%%%%%%%%%%%%%%%%%
  %% Addresses                                %%
  %%%%%%%%%%%%%%%%%%%%%%%%%%%%%%%%%%%%%%%%%%%%%%
  \address[A]{SAMOVAR,
  Télécom SudParis, Institut Polytechnique de Paris, 91120 Palaiseau.
  \printead{e1,e3}}
  \address[B]{LPSM, Sorbonne Université, UMR CNRS 8001, 4 Place Jussieu, 75005 Paris.
  \printead{e2}}
  \end{aug}

  \tableofcontents
  
  \input{suppl/proofthm1.tex}
  \input{suppl/proofthm2.tex}
  \input{suppl/proofprop1.tex}
  \input{suppl/algorithms.tex}
  \input{suppl/techres.tex}
  \input{suppl/predasymptvar.tex}
  \bibliographystyle{imsart-nameyear.bst}
  \bibliography{bibliography}
\end{document}
