# Supplementary material for: Variance estimation for Sequential Monte Carlo Algorithms: a backward sampling approach
Source: arXiv:2204.01401 source file (2023-01-02)
Supplement: Supplementary file 2 [file __latexindent_temp.tex]

    & F^N _{4,b} \eqdef \sum_{k^{1:4} _t \in [N]^4} \1_{k^1 _t \neq k^2 _t \neq k^3 _t \neq k^4 _t}  \sum_{k^{1:4} _{t-1} \in [N]^4} \prod_{\ell = 1}^4 \beta^\BS _t(k^\ell _t, k^\ell _{t-1}) \Pbacksum^b _{t-1}(k^1 _{t-1}, k^2 _{t-1}) \Pbacksum^b _{t-1}(k^3 _{t-1}, k^4 _{t-1}) \eqsp.
